# Supplementary material for: UltimateDO: An Efficient Framework to Marry Occupancy Prediction with 3D Object Detection via Channel2height
Source: arXiv:2409.11160 source file (2024-09-17)
Supplement: Supplementary file 1 [file supplement.tex]

\clearpage
\appendix
\section*{Appendix}

\section{Performance under various module setting}\label{Performance_under_various_module_setting}

We compared the performance of the model across different module configurations to identify the module that contributes most to performance. Table~\ref{tab:various_module_settings} provides a detailed breakdown of the model parameters for different configurations, and the specific precision of corresponding models are listed in Table~\ref{tab:performance_of_various_model}.

\begin{table*}[htb]
%\tiny
%\scriptsize
%\footnotesize
%\small
\normalsize
%\large
\setlength{\tabcolsep}{1.1mm}
\centering
\begin{tabular}{c|c|cc|c|cc|cc|c}
\toprule[1.5pt]   
\multicolumn{1}{c|}{\multirow{2}{*}{N.}} & \multirow{2}{*}{Size} & \multicolumn{2}{c|}{Image Encoder} & \multirow{2}{*}{View Transform} & \multicolumn{2}{c|}{BEV Encoder} & \multicolumn{2}{c|}{Head} & \multirow{2}{*}{G.}              \\ \cline{3-4} \cline{6-9}
\multicolumn{1}{c|}{}                      &                             & \multicolumn{1}{c|}{Bac.}  & Neck  &                                 & \multicolumn{1}{c|}{Bac.} & Neck & \multicolumn{1}{c|}{3D Detection} & Occupancy   \\ \cline{1-10}
M0 & 256$\times$704$\textcolor{white}{0}$ & \multicolumn{1}{c|}{R50$\textcolor{white}{0}$} & FL-256 & LSS-64,128$\times$128,1.0 & \multicolumn{1}{c|}{3b-128-256-512} & FL-256 & \multicolumn{1}{c|}{CenterPoint} & MH-128-256-288 & c \\ 
M1 & 256$\times$704$\textcolor{white}{0}$ & \multicolumn{1}{c|}{R50$\textcolor{white}{0}$} & FL-256 & LSS-64,128$\times$128,0.5 & \multicolumn{1}{c|}{3b-128-256-512} & FL-256 & \multicolumn{1}{c|}{CenterPoint} & MH-128-256-288 & c \\ 
M2 & 256$\times$704$\textcolor{white}{0}$ & \multicolumn{1}{c|}{R50$\textcolor{white}{0}$} & FL-256 & LSS-64,128$\times$128,0.5 & \multicolumn{1}{c|}{3b-128-256-512} & FL-256 & \multicolumn{1}{c|}{CenterPoint} & MH-256-512-288 & c \\ 
M3 & 256$\times$704$\textcolor{white}{0}$ & \multicolumn{1}{c|}{R50$\textcolor{white}{0}$} & FL-256 & LSS-64,256$\times$256,0.5 & \multicolumn{1}{c|}{3b-128-256-512} & FL-256 & \multicolumn{1}{c|}{CenterPoint} & MH-256-512-288 & c \\ 
M4 & 512$\times$1408 & \multicolumn{1}{c|}{R101} & FL-256 & LSS-64,128$\times$128,1.0 & \multicolumn{1}{c|}{3b-128-256-512} & FL-256 & \multicolumn{1}{c|}{CenterPoint} & MH-128-256-288 & c \\ 
M5 & 512$\times$1408 & \multicolumn{1}{c|}{R101} & FL-256 & LSS-64,256$\times$256,0.5 & \multicolumn{1}{c|}{3b-128-256-512} & FL-256 & \multicolumn{1}{c|}{CenterPoint} & MH-256-512-288 & c \\ 
M6 & 512$\times$1408 & \multicolumn{1}{c|}{R101} & FL-256 & LSS-64,128$\times$128,1.0 & \multicolumn{1}{c|}{3b-128-256-512} & FL-256 & \multicolumn{1}{c|}{CenterPoint} & MH-128-256-288 & b \\ 
\bottomrule[1.5pt]
\end{tabular}
\caption{Various module settings. The suffix "-number" signifies the count of channels within this module, while "number$\times$number" denotes the size of image or feature. "N.", "Bac." and "G." are short for name, backbone and graft category.
The letters "a", "b", and "c" in the row of "G." indicate the respective locations of the occupancy branch as illustrated in Figure~\ref{fig:illustration_of_occupancy_branch_grafted_on}.
}
\label{tab:various_module_settings}
\end{table*}

\begin{table*}[htb]
\setlength{\tabcolsep}{4.5mm}
\centering
\begin{tabular}{c|c|c|c|c|c|c|c}
\toprule[1.5pt]
\multicolumn{1}{c|}{\multirow{2}{*}{Name}} & \multirow{2}{*}{mIoU} & \multirow{2}{*}{mAP} & \multirow{2}{*}{NDS} & \multicolumn{3}{c|}{FPS/Time-consumption(ms)} & \multirow{2}{*}{Time-increment(ms)} \\ \cline{5-7} 
\multicolumn{1}{c|}{} & & & & \multicolumn{1}{c|}{Det.}  & Occ.  & \multicolumn{1}{c|}{Det.+Occ.} &    \\ \cline{1-8}
M0 & 31.0 & 28.9 & 36.4 & 205.63/4.86 & 194.63/5.13 & 181.10/5.52 & /$\%$ \\ 
M1 & 31.0 & 29.0 & 36.7 & 202.19/4.94 & 192.67/5.19 & 179.65/5.57 & 0.3/\textcolor{white}{0}6.1$\%$ \\ 
M2 & 31.1 & 29.4 & 36.7 & 202.11/4.94 & 176.40/5.66 & 166.03/6.02 & 1.1/22.4$\%$ \\ 
M3 & 32.2 & 29.7 & 36.8 & 125.23/7.98 & 123.72/8.08 & 110.39/9.05 & 0.2/2.5$\%$ \\ 
M4 & 35.4 & 36.6 & 43.6 & 30.43/32.86 & 30.29/33.01 & 29.98/33.35 & /$\%$ \\ 
M5 & 36.5 & 37.3 & 41.6 & / & / & / & /$\%$ \\ 
\bottomrule[1.5pt]
\end{tabular}
\caption{Performance of various module settings. 
"Det." and "Occ." denote 3D object detection and occupancy prediction respectively. .}
\label{tab:various_module_settings}
\end{table*}
